# Supplementary material for: EgoLife: Towards Egocentric Life Assistant
Source: arXiv:2503.03803 source file (2026-02-09)
Supplement: Supplementary file 1 [file appendix_demo.tex]

\section{More Qualitative Results}
